# Supplementary material for: Factorization in Call-by-Name and Call-by-Value Calculi via Linear Logic (long version)
Source: arXiv:2101.08364 source file (2021-01-20)
Supplement: Supplementary file 1 [file appendix.tex]

%\section*{Technical Appendix}

\input{embeddingNew-proofs}
\input{factorization-proofs}
